# Supplementary material for: Final Result on the Neutrinoless Double Beta Decay of $^{82}$Se with CUPID-0
Source: arXiv:2206.05130 source file (2022-06-10)
Supplement: Supplementary file 1 [file CUPID0_Final_Suppl.pdf]

# Supplemental Material for "Final Result on the Neutrinoless Double Beta Decay of $^{82}$Se with CUPID-0"

## DECAY SCHEME

Figure 1 shows a pictorial view of the decay scheme of $^{82}$Se to the fundamental and first excited states of its daughter, $^{82}$Kr.

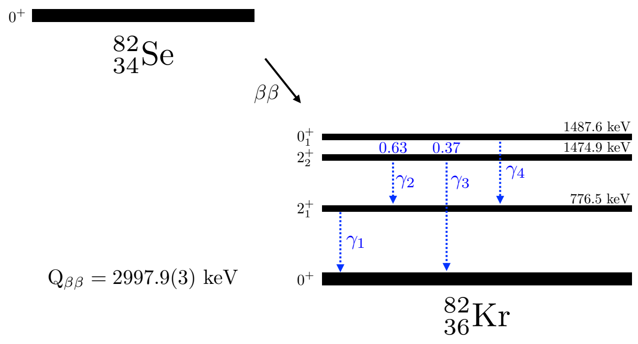


FIG. 1: Decay scheme of $^{82}$Se to $^{82}$Kr.

## FINAL PHYSICS SPECTRUM

Figure 2 shows the physics spectrum of CUPID-0 with a total $^{82}$Se exposure of 8.82 kg×yr (16.59 kg×yr in ZnSe). The only visible peaks are ascribed to $^{65}$Zn, $^{40}$K and $^{208}$Tl. $^{65}$Zn is produced by activation of the $^{64}$Zn naturally present in ZnSe crystals and decays with a half-life of ∼244 days. This isotope emits a $\gamma$-ray at 1115.5 keV and X-rays at 8.0 and 8.9 keV. The continous spectrum extending up to ∼3 MeV is dominated by the 2$\nu$DBD of $^{82}$Se.

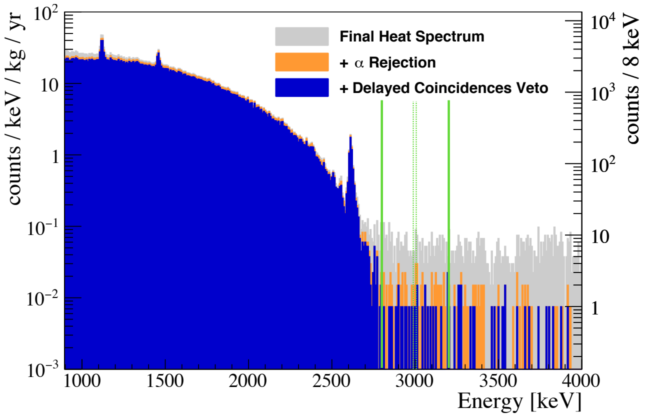


FIG. 2: Physics spectrum obtained with a $^{82}$Se exposure of 8.82 kg×yr (16.59 kg×yr in ZnSe). Grey: spectrum after a selection based on the quality of bolometric pulses and requiring that a single ZnSe detector triggered the event. Orange: same spectrum after rejecting $\alpha$ events. Blue: events surviving the delayed coincidence veto with potential $^{212}$Bi mothers. Green dotted lines: 1 FWHM centered around the $^{82}$Se Q-value; green vertical lines: region of interest for the evaluation of the background index (±200 keV window around the $^{82}$Se Q-value).

## ENERGY RESOLUTION

Figure 3 shows the energy resolution of the most prominent $\gamma$ peaks as a function of the energy. For this study we used the peaks produced by periodic calibrations with $^{232}$Th sources at 583 keV, 911 keV, 965+969 keV (modelled as a two peaks with the same RMS and with fixed means and amplitude ratios because of the finite energy resolution of the detector), 2615 keV.

In addition, we included two peaks that were observed in the physics spectrum of CUPID-0 and ascribed to $^{65}$Zn and $^{40}$K. Both these isotopes were modelled using a peak at the nominal energy of the $\gamma$-ray and a second peak with the same RMS, but with mean value fixed to the energy of $\gamma$+X-rays. The amplitude ratio of the two peaks was a free parameter of the fit.

As already described in Refs. [1–3], these peaks were not modelled using a single Gaussian, which is usually not satisfactory in describing a monochromatic energy deposit in bolometric detectors [4, 5]. On the contrary, we used a double Gaussian $\mathcal{G}(\mu_p, \sigma_p, \rho, \eta, \epsilon)$ where $\mu_p$ and $\sigma_p$ are the mean and RMS of the primary peak, and $\rho$, $\eta$, $\epsilon$ are the ratio of the mean, RMS and amplitude of the secondary to the primary Gaussian, respectively.

As shown in Figure 3, the simplest model describing the dependence of the FWHM on the energy is a linear function. This was expected, as in the past we conducted a dedicated study with a $^{56}$Co source emitting many peaks in the region of interest and, also in this large-statistics scenario, we observed a linear dependence [6]. While some experiments based on cryogenic calorimeters show the same behaviour [7, 8], others (e.g., CUORE, CUPID-Mo) require slightly more complex functions to model the dependence of the FWHM on the energy [9, 10].

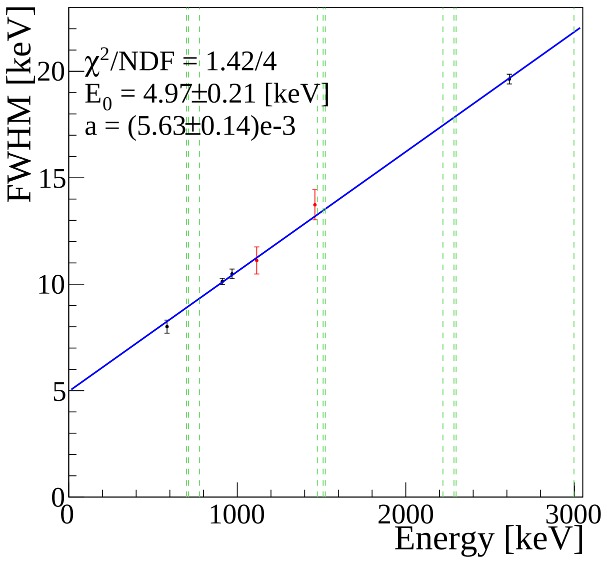


FIG. 3: FWHM of the most prominent peaks in calibration (black) and physics (red) runs. Blue line: fit function FWHM(E) = $E_0$ + a·E. Green dashed lines: energies of interest for the decay to the ground and excited states.

## SEARCH FOR THE $^{82}$SE DECAY TO THE EXCITED STATES OF $^{82}$KR: DATA FIT RESULTS

The events associated with each signature are saved into seven histograms (see main text), shown in the attached Figures. In each Figure, the region of interest is marked with red dashed lines and the fit result is shown with a continuous blue line.

The number of 0$\nu$DBD signal events ($N_i^{sig}$) can be written as

$$N_i^{sig} = \xi \cdot \varepsilon_i \cdot \Gamma_i \tag{1}$$

Where the total CUPID-0 exposure (phase-I + phase-II) is $\xi = 6.47 \times 10^{25}$ emitters × yr, the detection efficiency $\varepsilon_i$ is computed as the product of the data selection efficiency (see main text) by the containment efficiencies calculated with a Monte Carlo simulation (Table I in the main text), and $\Gamma_i$ is the decay width.

The searched signal was modelled using a double Gaussian $\mathcal{G}(\mu_p, \sigma_p, \rho, \eta, \epsilon)$ with mean values fixed to the nominal values of $E_{main}$. The FWHM were fixed to the values extracted from the fit (Figure 3). The background was modelled with a flat contribution ($N^{bkg}$) and, for signatures B, D, F and G, also with a peaking background at the nominal energy of the $^{40}$K peak ($\mathcal{G}(^{40}K)$).

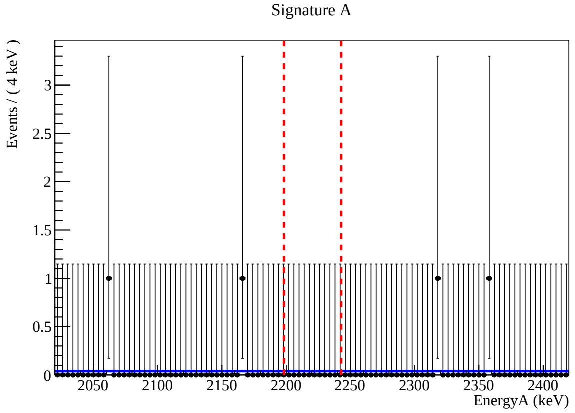


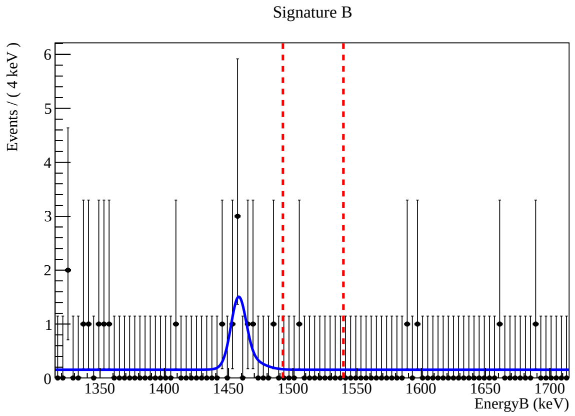


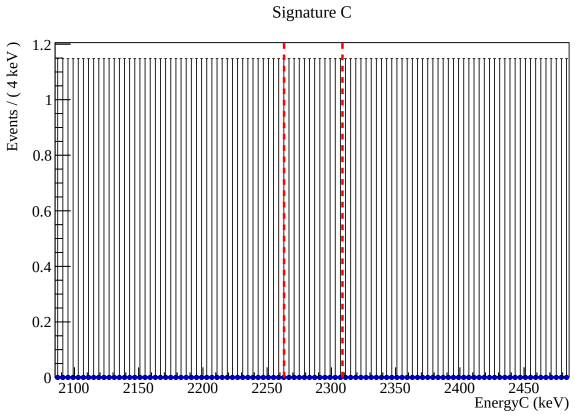


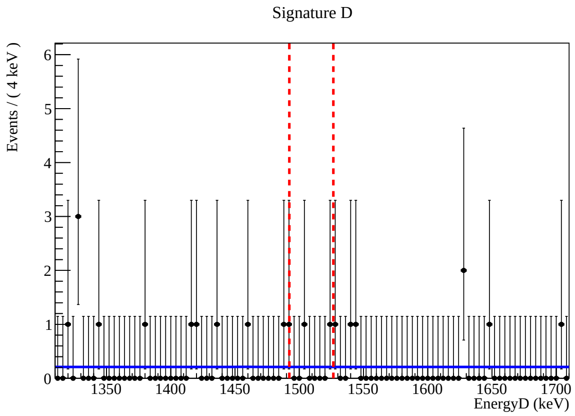

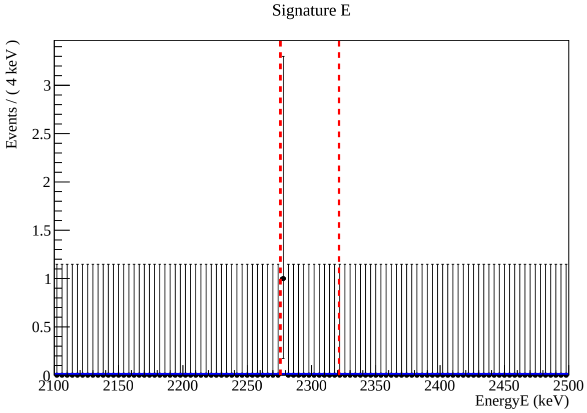


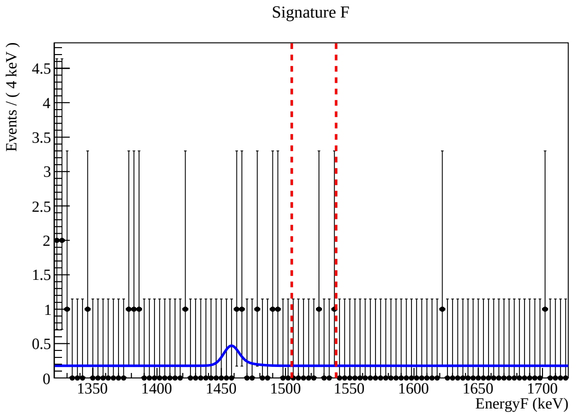


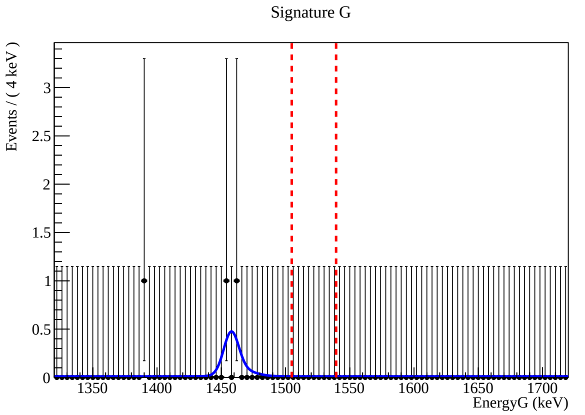


We can thus write the fit functions as:

$$f_A = N_A^{sig}\mathcal{G}(\mu = 2221.4\,\text{keV}, \sigma = 7.41\,\text{keV}) + N_A^{bkg} \tag{2a}$$

$$\begin{aligned} f_B = {} & N_{B1}^{sig}\mathcal{G}(\mu = 1510.3\,\text{keV}, \sigma = 5.71\,\text{keV}) \\ & + N_{B2}^{sig}\mathcal{G}(\mu = 1523.0\,\text{keV}, \sigma = 5.75\,\text{keV}) \\ & + N_B^{40}\mathcal{G}\left({}^{40}K\right) + N_B^{bkg} \end{aligned} \tag{2b}$$

$$f_C = N_C^{sig}\mathcal{G}(\mu = 2286.8\,\text{keV}, \sigma = 7.57\,\text{keV}) + N_C^{bkg} \tag{2c}$$

$$\begin{aligned} f_D = {} & N_D^{sig}\mathcal{G}(\mu = 1510.3\,\text{keV}, \sigma = 5.71\,\text{keV}) \\ & + N_D^{40}\mathcal{G}\left({}^{40}K\right) + N_D^{bkg} \end{aligned} \tag{2d}$$

$$f_E = N_E^{sig}\mathcal{G}(\mu = 2299.5\,\text{keV}, \sigma = 7.60\,\text{keV}) + N_E^{bkg} \tag{2e}$$

$$\begin{aligned} f_F = {} & N_F^{sig}\mathcal{G}(\mu = 1523.0\,\text{keV}, \sigma = 5.75\,\text{keV}) \\ & + N_F^{40}\mathcal{G}\left({}^{40}K\right) + N_F^{bkg} \end{aligned} \tag{2f}$$

$$\begin{aligned} f_G = {} & N_G^{sig}\mathcal{G}(\mu = 1523.0\,\text{keV}, \sigma = 5.75\,\text{keV}) \\ & + N_G^{40}\mathcal{G}\left({}^{40}K\right) + N_G^{bkg} \end{aligned} \tag{2g}$$

The numbers of events $N_i^{bkg}$ and $N_i^{40}$ are free parameters of the fit and, as explained in the main text, they can be written as a function of the decay widths $\Gamma_i$. The fit results are shown in the previous Figures.


[1] O. Azzolini *et al.* (CUPID-0), Phys. Rev. Lett. **120**, 232502 (2018), arXiv:1802.07791 [nucl-ex].

[2] O. Azzolini *et al.* (CUPID), Phys. Rev. Lett. **123**, 032501 (2019), arXiv:1906.05001 [nucl-ex].

[3] O. Azzolini *et al.*, Eur. Phys. J. **C78**, 734 (2018), arXiv:1806.02826 [physics.ins-det].

[4] C. Alduino *et al.* (CUORE), Phys. Rev. C **93**, 045503 (2016), arXiv:1601.01334 [nucl-ex].

[5] N. Casali *et al.*, J. Phys. G **41**, 075101 (2014), arXiv:1311.2834 [nucl-ex].

[6] O. Azzolini *et al.* (CUPID), Eur. Phys. J. **C78**, 888 (2018), arXiv:1807.00665 [nucl-ex].

[7] C. Alduino *et al.*, Physical Review C **93** (2016), 10.1103/physrevc.93.045503.

[8] S. Nagorny *et al.*, Nucl. Instr. and Meth. in Phys. Res. A **977**, 164160 (2020).

[9] D. Adams *et al.* (CUORE collaboration), Physical Review Letters **124** (2020), 10.1103/physrevlett.124.122501.

[10] B. Schmidt (CUPID-Mo collaboration), Journal of Physics: Conference Series **1468**, 012129 (2020).
